# Supplementary material for: Augmenting Human Expertise in Weighted Ensemble Simulations through Deep Learning based Information Bottleneck
Source: arXiv:2406.14839 ancillary file (2024-11-15)
Supplement: Supplementary file 1 [file SPIB_WE_SI.pdf]

# Supporting Information

## Augmenting Weighted Ensemble Simulations through Information Bottleneck

Dedi Wang<sup>1</sup> and Pratyush Tiwary<sup>\*1,2,3</sup>

<sup>1</sup>Biophysics Program and Institute for Physical Science and Technology, University of Maryland, College Park 20742, USA

<sup>2</sup>Department of Chemistry and Biochemistry and Institute for Physical Science and Technology, University of Maryland, College Park 20742, USA

<sup>3</sup>University of Maryland Institute for Health Computing, Bethesda 20852, USA.

### 1 Supplementary Methods

#### 1.1 State Predictive Information Bottleneck (SPIB)

For weighted ensemble (WE) simulations, a set of short trajectory segments are collected for the State Predictive Information Bottleneck (SPIB) training. For given  $M$  short trajectories with length of  $L$ ,  $\{\mathbf{X}^{m,1}, \dots, \mathbf{X}^{m,L}\}_{m=1}^M$  and the corresponding state labels  $\{\mathbf{y}^{m,1}, \dots, \mathbf{y}^{m,L}\}_{m=1}^M$ , where the state labels can be learned on the fly in SPIB,<sup>[3, 2]</sup> along with the associated weights for each trajectory segment  $\{w^m\}_{m=1}^M$  obtained from WE simulations, the objective function of SPIB can be formulated as:

$$\begin{aligned} \operatorname{argmax}_{\theta} \mathcal{L}(\theta) = \\ \sum_{m=1}^M \frac{w^m}{\sum_{j=1}^M w^j} \frac{1}{L-s} \sum_{n=1}^{L-s} \left[ \log q_{\theta}(\mathbf{y}^{m,n+s} | \mathbf{z}^{m,n}) - \beta \log \frac{p_{\theta}(\mathbf{z}^{m,n} | \mathbf{X}^{m,n})}{r_{\theta}(\mathbf{z}^{m,n})} \right] \end{aligned} \quad (1)$$

where the encoder  $p_{\theta}(\mathbf{z} | \mathbf{X})$ , the decoder  $q_{\theta}(\mathbf{y} | \mathbf{z})$ , and the prior  $r_{\theta}(\mathbf{z})$  are probability distributions parameterized by deep neural networks  $\theta$ .  $\mathbf{z}^{m,n}$  is sampled from  $p_{\theta}(\mathbf{z} | \mathbf{X}^{m,n})$  and the time interval between  $\mathbf{X}^{m,n}$  and  $\mathbf{X}^{m,n+s}$  is the lag time  $\Delta t$ , or how far into the future SPIB should predict. The first term  $\log q_{\theta}(\mathbf{y}^{m,n+s} | \mathbf{z}^{m,n})$  measures the ability of our representation to predict the desired target, while the second term  $\log \frac{p_{\theta}(\mathbf{z}^{m,n} | \mathbf{X}^{m,n})}{r_{\theta}(\mathbf{z}^{m,n})}$  can be interpreted as the complexity penalty that acts as a regulariser. This regularization term encourages the latent space  $\mathbf{z}$  to follow the prior distribution  $r_{\theta}(\mathbf{z})$  and retain less information from the input  $\mathbf{X}$ , thereby promoting a more compact representation. Such a trade-off between the prediction capacity and model complexity is then controlled by a hyperparameter  $\beta \in [0, \infty)$ . For a detailed discussion of the choice of the encoder  $p_{\theta}(\mathbf{z} | \mathbf{X})$ , the decoder  $q_{\theta}(\mathbf{y} | \mathbf{z})$ , and the prior  $r_{\theta}(\mathbf{z})$ , readers can refer to the recent publication.<sup>[2]</sup>

To ensure a more uniform CV space for binning, we find the regularization term in [2](#) plays a crucial role. As detailed in Ref. [\[2\]](#), we employ a mixture of Gaussians with the same variance as the prior. For example, if SPIB identifies  $S$  states, then we will assume the learned CVs should follow a mixture of  $S$  Gaussians with the same variance. Such a prior in principle should enable the learning of a CV space with enhanced

---

\*Email: ptiwary@umd.edu

homogeneity. However, in practice, since the regularization term is weighted by the weights associated with each state, it may fail to regularize the CVs for states with small populations to follow Gaussians with the same variance. This is because the deviation of those states from the prior may not significantly contribute to the regularization term. To better regularize the learned CVs and allow states with small populations to still contribute to the regularization term, we decide to reweight the regularization term to ensure that each state has an equal contribution:

$$\begin{aligned} \operatorname{argmax}_{\theta} \mathcal{L}(\theta) = \\ \sum_{m=1}^M \sum_{n=1}^{L-s} \left[ \frac{w^m}{\sum_{j=1}^M w^j} \frac{1}{L-s} \log q_{\theta}(\mathbf{y}^{m,n+s} | \mathbf{z}^{m,n}) - \beta c^{m,n} \log \frac{p_{\theta}(\mathbf{z}^{m,n} | \mathbf{X}^{m,n})}{r_{\theta}(\mathbf{z}^{m,n})} \right], \end{aligned} \quad (2)$$

where  $c^{m,n} = \sum_{i=1}^S \frac{\mathbb{1}_{\mathbf{y}^{m,n}=i} w^m}{\sum_{m=1}^M \sum_{n=1}^{L-s} \mathbb{1}_{\mathbf{y}^{m,n}=i} w^m}$  is the new weight assigned to samples within each state in the regularization term, calculated by reweighting the samples based on the total weights within each state.  $\mathbb{1}_{\mathbf{y}^{m,n}=i}$  is the indicator function, returning 1 only if the state label  $\mathbf{y}^{m,n} = i$ , and 0 otherwise. It's important to note that we only reweight the regularization term, leaving the first term  $\log q_{\theta}(\mathbf{y}^{m,n+s} | \mathbf{z}^{m,n})$  untouched, as we aim for the model to unbiasedly predict the dynamics.

## 1.2 Model Binning Scheme

in this work, To bin the learned CVs, we employ a rectilinear grid with equal bin sizes to uniformly bin the SPIB-learned CV space. A simple iterative algorithm is used to automatically adjust the bin size, aiming to maintain a roughly constant desired number of occupied SPIB bins, as show in Alg. 1. In this work, we set the desired number of occupied SPIB bins to 100 for both alanine and CLN025 systems, and the tolerance  $tol = 0.1$ .

---

### Algorithm 1 Determine the bin size for the SPIB learned CVs

---

**Input:** the final SPIB learned CVs of all segments within the current WE iteration  $\{\mathbf{z}^m\}_{m=1}^M$ , the desired number of occupied SPIB bins  $n_{occupied}$ , the tolerance  $tol$

- 1: Get the dimension of the SPIB learned CVs  $d_z$
  - 2: Get the maximum and minimum values of the SPIB learned CVs along each dimension,  $\{z_{i,max}, z_{i,min}\}_{i=1}^{d_z}$ , from the samples  $\{\mathbf{z}^m\}_{m=1}^M$
  - 3:  $h_{bin} \leftarrow \left[ \prod_{i=1}^{d_z} |z_{i,max} - z_{i,min}| \right]^{1/d_z}$
  - 4: Uniformly grid the CVs  $\mathbf{z}$  using the rectilinear grid with the bin size  $h_{bin}$
  - 5:  $\hat{n}_{occupied} \leftarrow$  count the number of occupied bins using samples  $\{\mathbf{z}^m\}_{m=1}^M$
  - 6: **while**  $|\hat{n}_{occupied} - n_{occupied}|/n_{occupied} < tol$  **do**
  - 7:    $h_{bin} \leftarrow \left[ \frac{\hat{n}_{occupied}}{n_{occupied}} h_{bin}^{d_z} \right]^{1/d_z}$
  - 8:   Uniformly grid the CVs  $\mathbf{z}$  using the rectilinear grid with the new bin size  $h_{bin}$
  - 9:    $\hat{n}_{occupied} \leftarrow$  count the number of occupied bins using samples  $\{\mathbf{z}^m\}_{m=1}^M$
  - 10: **end while**
  - 11: Return the final rectilinear grid and its bin size  $h_{bin}$
- 

## 1.3 Model Architecture and Training

In this study, both the encoder and decoder of SPIB are nonlinear and parameterized by fully connected neural networks consisting of two hidden layers. A rectified linear unit (ReLU) serves as the activation function for all hidden layers. Each hidden layer in both the encoder and decoder comprises 32 nodes. The dimensionality of the learned CVs is set to 2, with a lag time of  $\Delta t = 10$  ps, and  $\beta = 0.01$ . To train the model, Adam optimizers with a learning rate of 0.001 are employed for training the neural networks. We set the batch size to 4096, the tolerance to 0.001, the patience to 2, and the number of refinements to 15.

To initialize the state labels for SPIB training, we discretize the expert-based CVs through regular space clustering [1] using the Euclidean distance metric, resulting in approximately 100 clusters. The determination of the minimum cluster-cluster distance follows a process similar to that outlined in Algorithm 1.

## References

- [1] Jan-Hendrik Prinz, Hao Wu, Marco Sarich, Bettina Keller, Martin Senne, Martin Held, John D Chodera, Christof Schütte, and Frank Noé. Markov models of molecular kinetics: Generation and validation. *The Journal of chemical physics*, 134(17):174105, 2011.
- [2] Dedi Wang, Yunrui Qiu, Eric Beyerle, Xuhui Huang, and Pratyush Tiwary. An information bottleneck approach for markov model construction. *arXiv preprint arXiv:2404.02856*, 2024.
- [3] Dedi Wang and Pratyush Tiwary. State predictive information bottleneck. *The Journal of Chemical Physics*, 154(13):134111, 04 2021.
